# Supplementary material for: A Reusable Library for Second-Order Orbital Optimization Using the Trust Region Method
Source: arXiv:2509.13931 ancillary file (2025-11-10)
Supplement: Supplementary file 1 [file si.pdf]

# Supporting Information:

## A Reusable Library for Second-Order Orbital Optimization Using the Trust Region Method

Jonas Greiner,<sup>\*,†</sup> Ida-Marie Høyvik,<sup>\*,‡</sup> Susi Lehtola,<sup>\*,¶</sup> and Janus J. Eriksen<sup>\*,†</sup>

<sup>†</sup>*DTU Chemistry, Technical University of Denmark*

*Kemitorvet Bldg. 206, 2800 Kgs. Lyngby, Denmark*

<sup>‡</sup>*Department of Chemistry, Norwegian University of Science and Technology*

*Realfagbygget, D3-139, Trondheim 7491, Norway*

<sup>¶</sup>*Department of Chemistry, University of Helsinki*

*P. O. Box 55, FIN-00014, Finland*

E-mail: [jongr@dtu.dk](mailto:jongr@dtu.dk); [ida-marie.hoyvik@ntnu.no](mailto:ida-marie.hoyvik@ntnu.no); [susi.lehtola@helsinki.fi](mailto:susi.lehtola@helsinki.fi); [janus@dtu.dk](mailto:janus@dtu.dk)

Table S1: Key hyperparameters used in the main study.

| Parameter                                                    | Value / Notes                                                                                                             |
|--------------------------------------------------------------|---------------------------------------------------------------------------------------------------------------------------|
| <i>Level-shift determination</i>                             |                                                                                                                           |
| Level-shifting criterion                                     | Lowest augmented Hessian eigenvalue $< -10^{-5}$                                                                          |
| Bisection lower bound $\alpha_{\min}$                        | $10^{-4}$                                                                                                                 |
| Bisection upper bound $\alpha_{\max}$                        | $10^6$                                                                                                                    |
| Bisection convergence criterion $\Delta\alpha_{\text{conv}}$ | $10^{-12}\alpha_{\text{upper}}$                                                                                           |
| <i>Micro-iterations</i>                                      |                                                                                                                           |
| Number of random starting vectors                            | 1                                                                                                                         |
| Orthogonalization of trial vectors                           | Iterations of modified Gram-Schmidt until floating-point precision                                                        |
| Preconditioner                                               | Diagonal (default); custom optional                                                                                       |
| Residual norm conv. criterion                                | Reduction by factor $10^{-3}$ in global region<br>Reduction by factor $10^{-4}$ in local region                           |
| Max. number of micro-iterations                              | 50                                                                                                                        |
| <i>Trust region control</i>                                  |                                                                                                                           |
| Initial trust region radius, $h_{\text{start}}$              | 0.4                                                                                                                       |
| Trust region reduction criterion                             | Ratio of actual to predicted reduction $< 0.25$                                                                           |
| Trust region reduction                                       | 0.7                                                                                                                       |
| Trust region expansion criterion                             | Ratio of actual to predicted reduction $> 0.75$                                                                           |
| Trust region expansion                                       | 1.2                                                                                                                       |
| <i>Line Search (Bracketing)</i>                              |                                                                                                                           |
| Bracketing                                                   | Optional when objective function evaluation is cheap                                                                      |
| Bracketing grow limit                                        | 110                                                                                                                       |
| <i>Macro-iterations</i>                                      |                                                                                                                           |
| Step rejection criteria                                      | Objective function increases<br>Maximum number of micro-iterations reached<br>Any orbital pair rotation $> \frac{\pi}{4}$ |
| Gradient RMS conv. criterion                                 | $10^{-5}$                                                                                                                 |
| Max. number of macro-iterations                              | 150                                                                                                                       |
| <i>Stability check</i>                                       |                                                                                                                           |
| Number of random starting vectors                            | 20                                                                                                                        |
| RMS Residual conv. criterion                                 | $10^{-8}$                                                                                                                 |
| Stability criterion                                          | Lowest Hessian eigenvalue $> -10^{-2}$                                                                                    |
| Max. number of iterations                                    | 100                                                                                                                       |

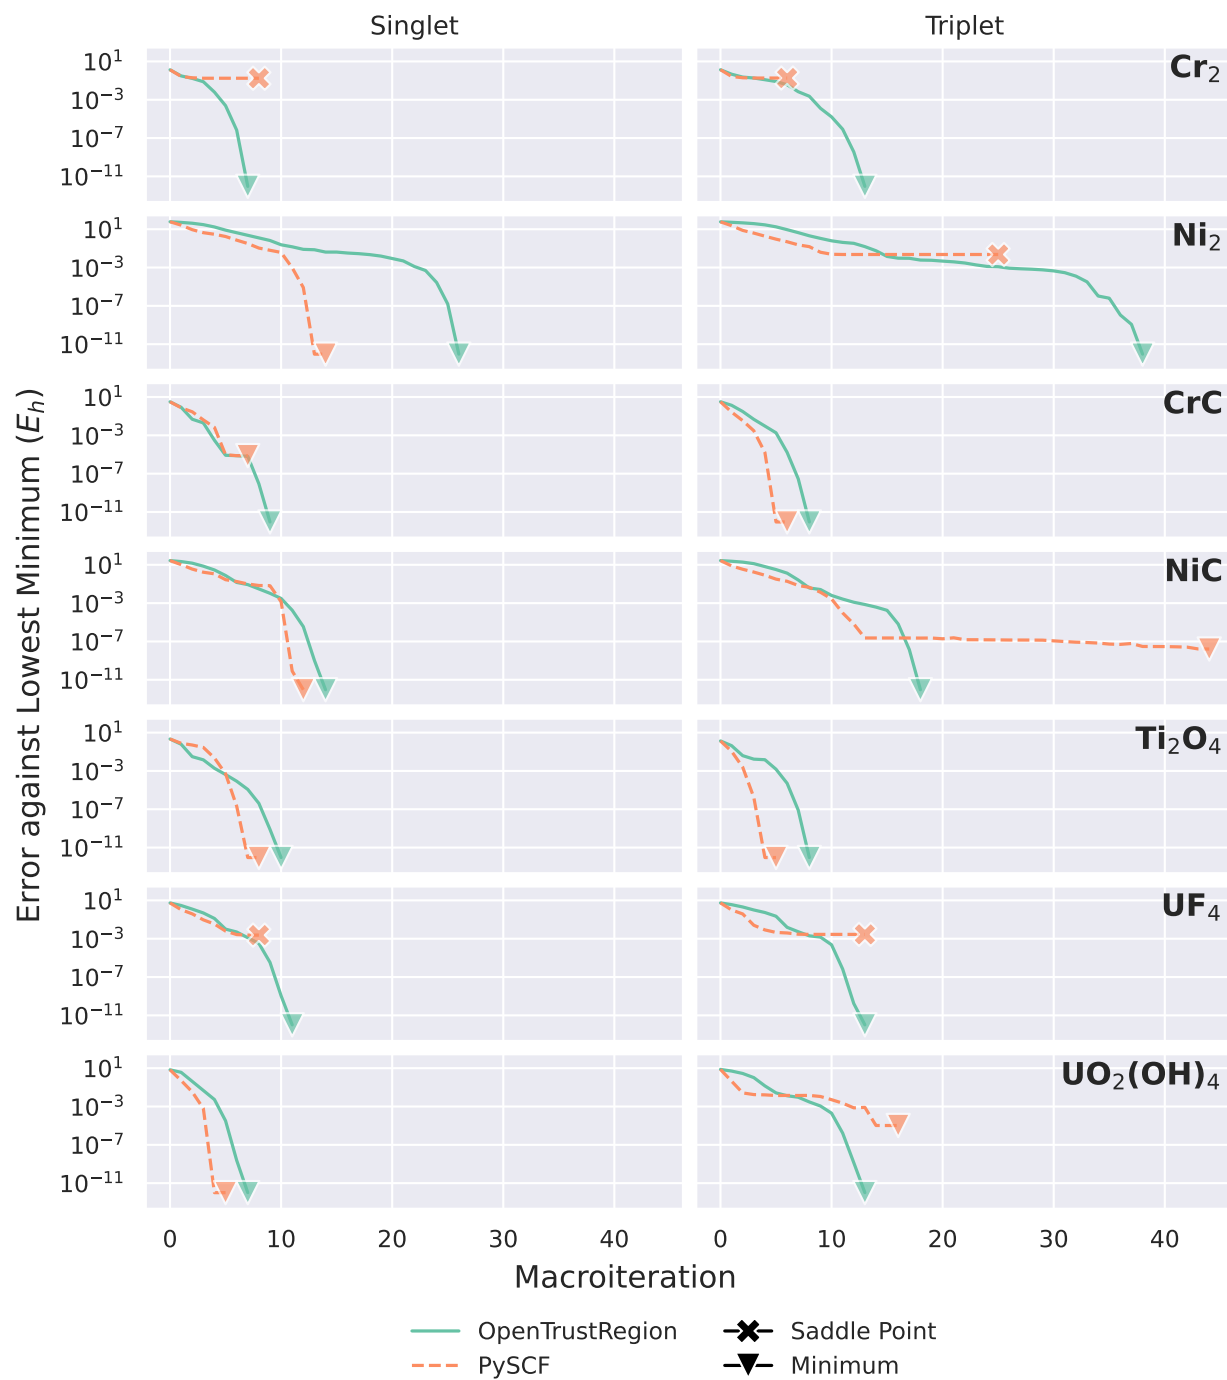

Figure S1: KS-DFT/PBE results on par with Fig. 2 of the main study.

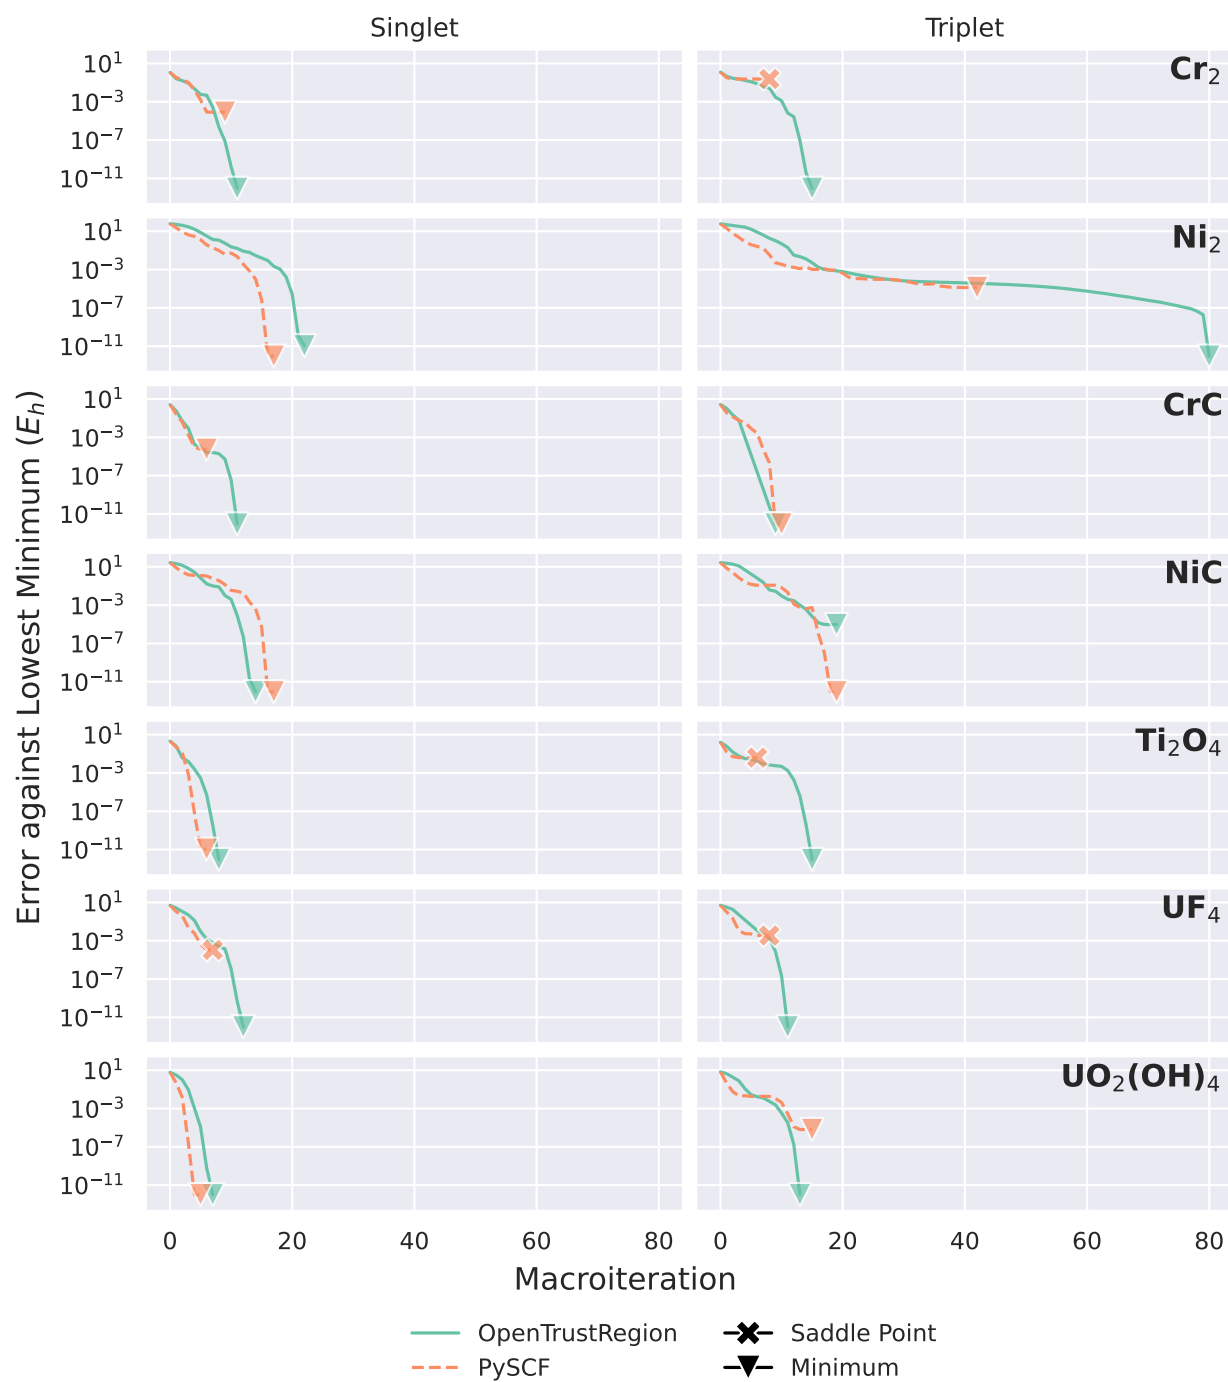

Figure S2: KS-DFT/B3LYP results on par with Fig. 2 of the main study.

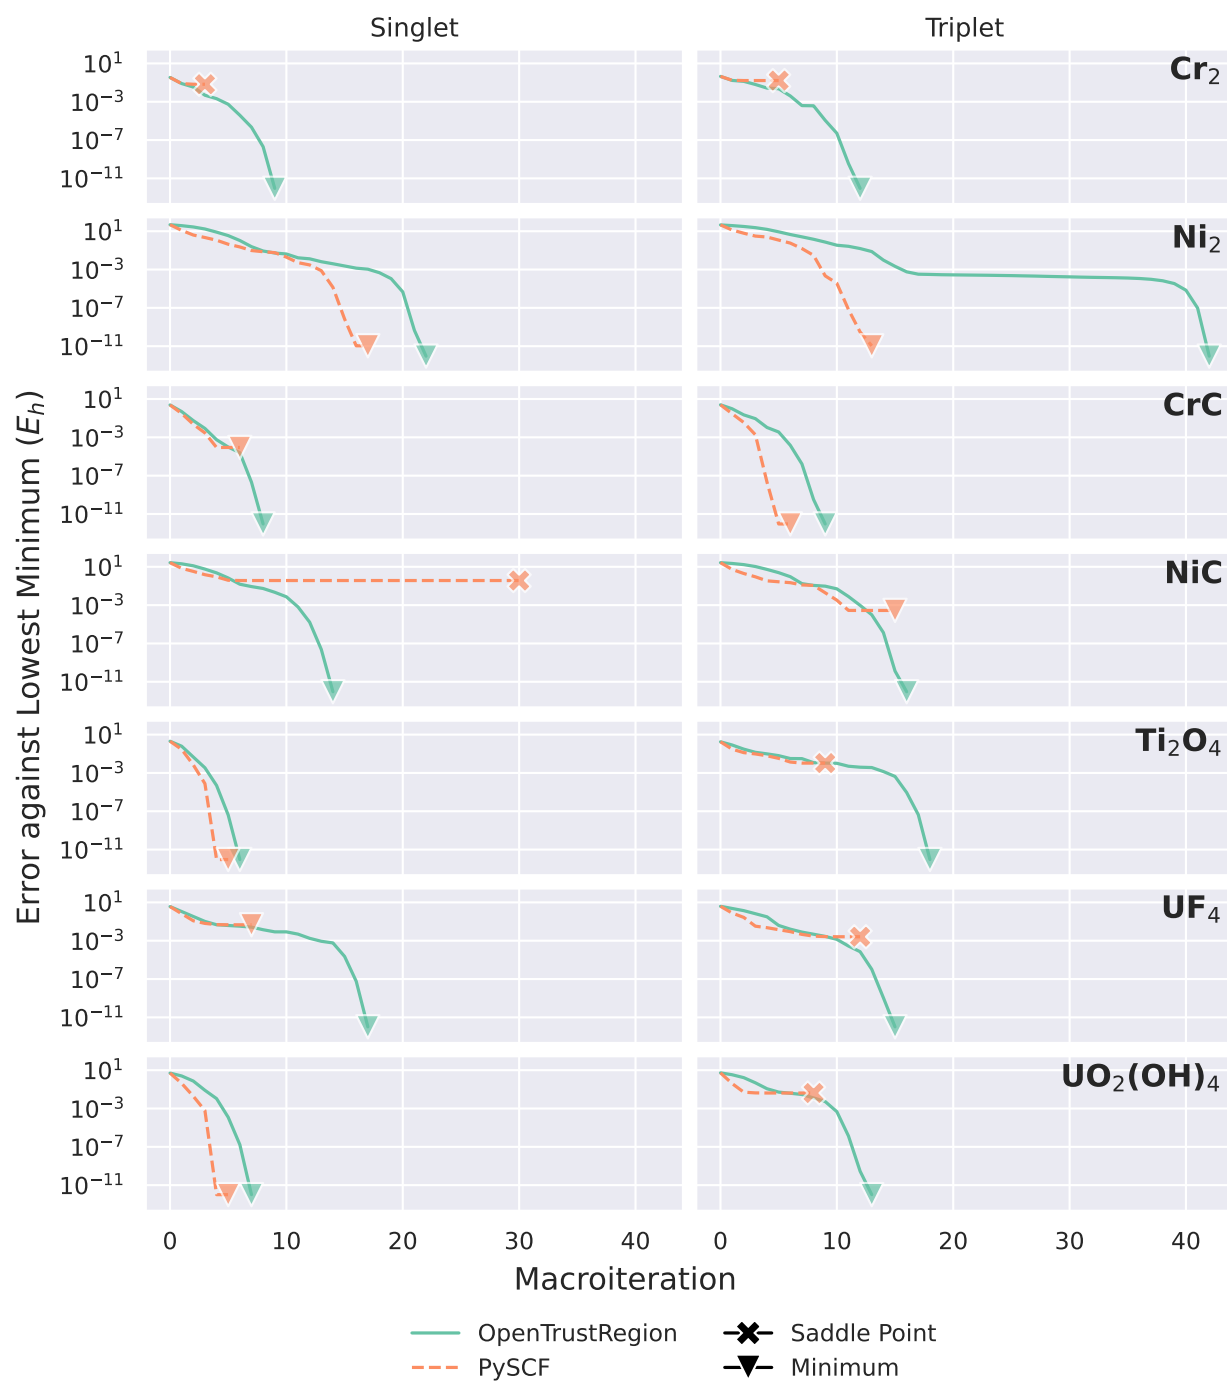

Figure S3: KS-DFT/ $\omega$ B97X results on par with Fig. 2 of the main study.

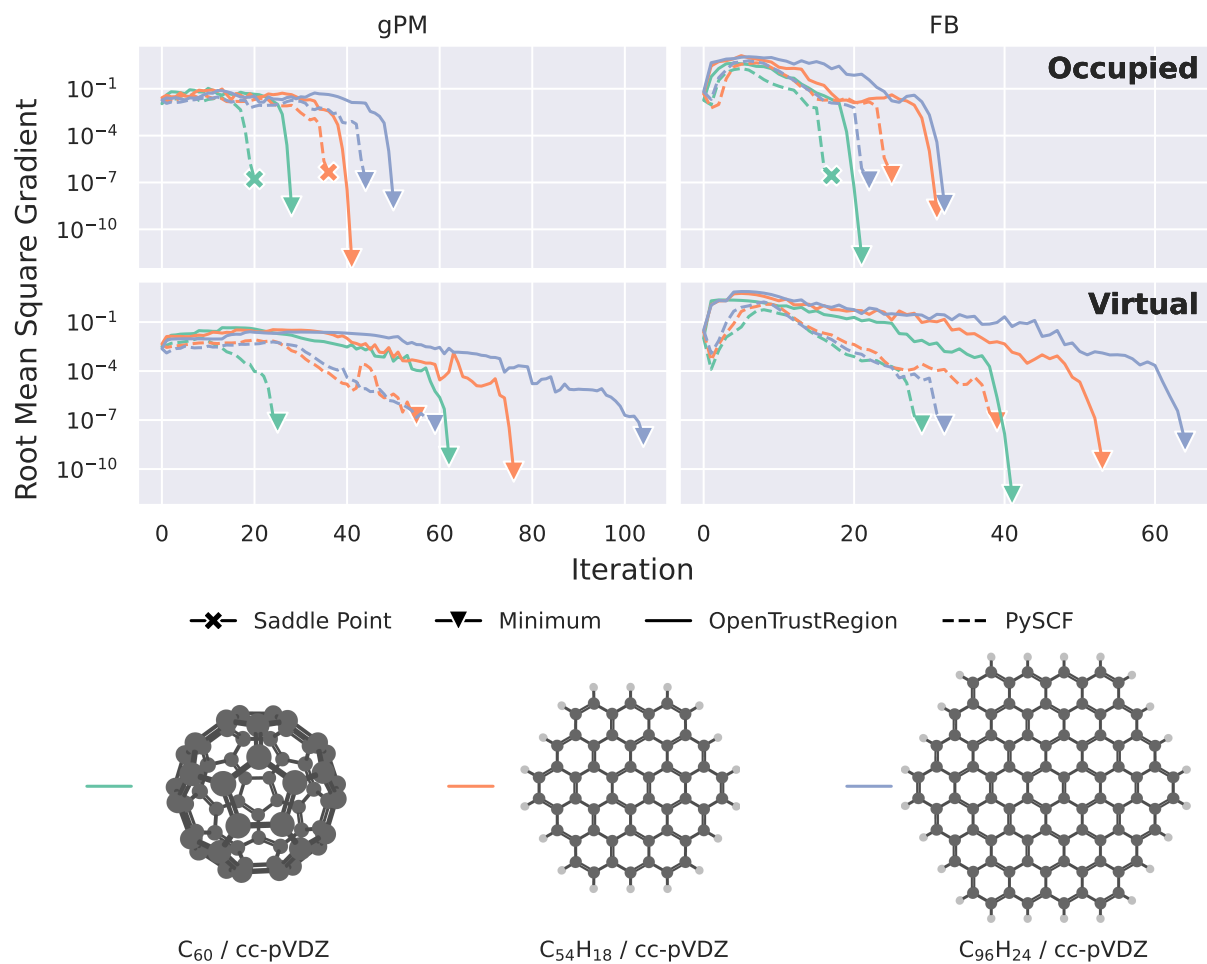

Figure S4: Same results as in Fig. 4 of the main study, but using a cc-pVDZ basis set.
